# Supplementary material for: Tensor Factorization via Matrix Factorization
Source: arXiv:1501.07320 source file (2015-05-18)
Supplement: Supplementary file 1 [file appendix.tex]

% DEPRECATED

\section{Proofs}

\begin{lemma}[Perturbation bound for eigenvectors]
  \begin{align*}
\| \vt_i - v_i \|_2 
&\leq \e \sqrt{\sum_{j \neq i} E_{ij}^2} + o(\e),
  \end{align*}
  where $E$ is a skew symmetric matrix such that
\end{lemma}

\begin{proof}
  From \lemmaref{cardoso} we have that the eigenvectors $\Vt$ returned
  by \algorithmref{jacobi} on the set of matrices $\hat\sM = \{\Mh_1, \dots, \Mh_L\}$ satisfy
  $
    \Vt = V(I + \e E + o(\e))
  $, 
Let $\Delta_{ij} = \pi_i v_i - \pi_j v_j$. Then $\lambda_{il} - \lambda_{jl} = w_l^\top \Delta_{ij}$.  
Then,
\begin{align*}
  E_{ij} 
  &= 
    \frac{\sum_{l=1}^L w_l^\top \Delta_{ij} R(v_i, v_j, w_l)}
    {\sum_{l=1}^L (w_l^\top \Delta_{ij})^2} \\
  &= 
  \frac{\sum_{l=1}^L w_l^\top \Delta_{ij} R_{ij} w_l}
    {\sum_{l=1}^L w_l^\top \Delta_{ij} \Delta_{ij}^\top w_l}.
\end{align*}

  This gives us that, 
$$ \vt_i = v_i + \epsilon \sum_{j \neq i} E_{ij} u_j + o(\e) $$
and consequently \pl{how does the last line follow? should it be an inequality?}
\begin{align*}
|| \vt_i - v_i ||^2_2 
  &\leq \e^2 \sum_{i \neq j} |E_{ij}|^2 + o(\e^2) \\
  &= 
    \e^2 \sum_{j \neq i} \left( \sum_{l=1}^L \frac{\lambda_{il} - \lambda_{jl}}{\sum_{l=1}^L (\lambda_{il} - \lambda_{jl})^2} v_j^\top R_l v_i \right)^2 
        + o(\e^2) \\
  &=
  \e^2 \sum_{j \neq i} \left( \frac{1}{\max_{l \in [L]} |\lambda_{il} - \lambda_{jl}|} \right)^2 \left( \sum_{l=1}^L  \frac{x_{jl}}{\sum_{l=1}^L x_{jl}^2}| v_j^\top R_l v_i | \right)^2 
        + o(\e^2),
\end{align*}
where $0 \geq x_{jl} \geq 1$ are defined as
\begin{align*}
x_{jl} &= \frac{|\lambda_{il} - \lambda_{jl}|}{\max_{l \in [L]} |\lambda_{il} - \lambda_{jl}|}.
\end{align*}

Finally, we get,
\begin{align*}
|| \vt_i - v_i ||_2^2
&\leq 
  \left(\e \max_{j \neq i} \min_{l \in [L]} \frac{1}{|\lambda_{il} - \lambda_{jl}|} \right)^2 
  \sum_{j \neq i} \left( \sum_{l=1}^L  \frac{x_{jl}}{\sum_{l=1}^L x_{jl}^2}| v_j^\top R_l v_i | \right)^2 
    + o(\e^2) \\
\end{align*}

Next, using Assumption \ref{asm:incoherence} and Lemma \ref{lem:maxbound}, we have
\begin{align*}
|| \vt_i - v_i ||_2^2
& \leq (\e \max_{j \neq i} \min_{l=1}^L  \frac{1}{|\lambda_{il} - \lambda_{jl}|}  ) ^2 \sum_{j \neq i} ( \sum_{l=1}^L  \frac{x_{jl}}{\sum_{l=1}^L x_{jl}^2} \frac{\kappa}{\sqrt{d}})^2 + o(\e) \\
& \leq (\e \max_{j \neq i} \min_{l=1}^L  \frac{1}{|\lambda_{il} - \lambda_{jl}|} ) ^2 \sum_{j \neq i} \frac{\kappa^2}{d} ( \sum_{l=1}^L  \frac{x_{jl}}{\sum_{l=1}^L x_{jl}^2}  )^2 + o(\e) \\
& \leq (\e \max_{j \neq i} \min_{l=1}^L  \frac{1}{|\lambda_{il} - \lambda_{jl}|} ) ^2 \sum_{j \neq i} \frac{\kappa^2}{d} C^2 + o(\e) \\
& \leq (\e \max_{j \neq i} \min_{l=1}^L  \frac{1}{|\lambda_{il} - \lambda_{jl}|} ) ^2 \cdot \kappa^2 \cdot C^2 + o(\e).
\end{align*}

\pl{spell it out more...where is $C$ defined?}
Our claim follows immediately using the additional observation that $\sqrt{x+y} \leq \sqrt{x} + \sqrt{y}$ for $x,y \geq 0$.

  Note that $M_l = T(I, I, w_l)$, and thus
  $\lambda_{il} = \mu_i w_l^\top v_i$.
\end{proof}

\begin{lemma}[Perturbation bound for eigenvectors]
  Let $\pit$ and $\vt$ be factorization of $\Th$ returned by \algorithmref{joint}.
  If $\e \le \frac{1}{d}$, then
  \begin{align*}
\| \vt_i - v_i \|_2 
  &\leq \frac{\e}{2 \pi_{\min}} \sum_{j \neq i \in [k]} \|R(v_i, v_j, I)\|_2^2 + o(\e).
  \end{align*}
\end{lemma}

\subsubsection{Analysis for random projections}

First, we state a technical lemma that shows that a random projection $w^\top v$ concentrates around $\Theta(1/\sqrt{d})$.

\pl{disambiguate bracketing: $(\ln \delta)^2$}
\begin{lemma}[Dasgupta and Gupta, 2003]
Let $w \in \mathbb R^d$ be a random vector distributed uniformly over the sphere $\mathcal S^{d-1}$, and fix a vector $v \in \mathbb R^d$.
\begin{enumerate}
\item If $\delta \in (0,1)$, then
$$ P( |w^\top v| \leq \frac{||v||_2}{\sqrt{d}} \delta ) \leq \exp( \frac{1}{2}(1-\delta^2 + \ln \delta^2) ). $$

\item If $\delta > 1$, then
$$ P( |w^\top v| \geq \frac{||v||_2}{\sqrt{d}} \delta ) \leq \exp( \frac{1}{2}(1-\delta^2 + \ln \delta^2) ). $$
\end{enumerate}
\end{lemma}

It is now easy to establish our main lemma for random projections.

\pl{use $\sigma$ or something instead of $\pi$ for the permutation to avoid clashing notation}
\pl{choose nicer numbers; really don't think you need $\sqrt{e}/2$}
\pl{it's clearer if you carry the $L_0$ to the very end, get an expression and then solve for the value
rather than substituting it half way through}
\begin{lemma}[Random projections]
Let $\vt_1\supr{0}, ..., \vt_n\supr{0}$ be the result of simultaneously diagonalizing $L_0 \geq  \lceil \log_{\sqrt{e}/2} \left( \delta / {{n \choose 2}} \right) \rceil$ random projections $T(I,I,w_l)$ for $l=1,...,L_0$ of tensor $T$, where each $w_l$ is chosen uniformly at random from the unit sphere $\mathcal S^{d-1}$. For some permutation $\pi$, with probability $1-\delta$, we have
$$ ||\vt_i\supr{0} - v_{\pi(i)}||_2 \leq \e \cdot C \cdot \kappa \cdot \frac{2 \sqrt{d}}{\pi_\textrm{min}} + o(\e). $$
\end{lemma}

\begin{proof}
From Lemma \ref{lem:maxmin}, we know that
$$ || \vt_i - v_i ||_2 \leq \e \cdot C \cdot \kappa \cdot \max_{j \neq i} \min_{l=1}^{L_0} \frac{1}{| w_l^\top (\pi_i v_i - \pi_j v_j)|} + o(\e). $$

Let $u_{ij} = \pi_i v_i - \pi_j v_j$ and observe that
\begin{align*}
P( \min_{l=1}^{L_0} \frac{1}{| w_l^\top (\pi_i v_i - \pi_j v_j)|} > \frac{2 \sqrt{d}}{||u_{ij}||_2} )
& \leq P( | w_l^\top u_{ij} | \leq ||u_{ij}||_2 \frac{0.5}{\sqrt{d}} )^{L_0} \\
& \leq \exp(\frac{1}{2} ( 1 - 0.5^2 + \ln(0.5) ) )^{L_0} \\
& \leq ( \sqrt{e}/2 ) ^{L_0} \\
& \leq ( \sqrt{e}/2 ) ^ {\log_{\sqrt{e}/2}(\delta / {n \choose 2})} \\
& = \delta / {n \choose 2}
\end{align*}

We can extend this bound to all pairs $i, j$ using the union bound and the observation that $||u_{ij}||_2 = ||\pi_i v_i - \pi_j v_j||_2 = \sqrt{\pi_i^2 + \pi_j^2} \geq \pi_\textrm{min}$:

\pl{shouldn't $j \le i$ be $j < i$?}
\begin{align*}
P \left(\max_{j \leq i} \min_{l=1}^{L} | \frac{1}{w_l^\top(v_i - v_j)} |  > \frac{2 \sqrt{d}}{\pi_\textrm{min}} \right) 
& = P \left(\exists i,j,  {j \leq i} \textrm{ s.t. } \min_{l=1}^{L} | \frac{1}{w_l^\top(v_i - v_j)} |  > \frac{2 \sqrt{d}}{\pi_\textrm{min}} \right) \\
& \leq P \left(\exists i,j,  {j \leq i} \textrm{ s.t. } \min_{l=1}^{L} | \frac{1}{w_l^\top(v_i - v_j)} |  > \frac{2 \sqrt{d}}{||u_{ij}||_2} \right) \\
& \leq \sum_{i,j : i \leq j} P \left(\min_{l=1}^{L} | \frac{1}{w_l^\top u_{ij}} |  > \frac{2 \sqrt{d}}{||u_{ij}||_2} \right) \\
& \leq \sum_{i,j : i \leq j} \delta / {n \choose 2} \\
& = \delta
\end{align*}

This establishes the desired result with probability $1-\delta$.
\end{proof}

\subsection{Analysis for deterministic projections}

\subsubsection{Analysis for non-random $w_l$}

First, we lower bound the gap $w_l^\top(v_i - v_j)$.
\pl{state relatinship between $w_l$, $\vt_i$, ...}
\pl{$\vt_i$ should be $\vt_i^{(0)}$?}

\begin{lemma}\label{lem:gaplowerbound}
Let $\vt_i \in \mathbb R^d$ be such that $||v_i - \vt_i|| \leq \delta$. Then for any $j\neq i$,
$$ \vt_i^\top (\pi_i v_i - \pi_j v_j) \geq 1 - \sqrt{2}\cdot\pi_\textrm{max} \cdot \delta. $$
\end{lemma}

\begin{proof}
  Observe that \pl{why is the first equality true?}
\begin{align*}
\vt_i^\top (v_i - v_j) & = (v_i +(v_i - v_i))^\top (\pi_i v_i - \pi_j v_j) \\
& = (v_i)^\top (\pi_i v_i - \pi_j v_j) + (\vt_i - v_i)^\top (\pi_i v_i - \pi_j v_j) \\
& \geq 1 - \sqrt{\pi_i^2 + \pi_j^2} \cdot \delta \\
& \geq 1 - \sqrt{2}\cdot\pi_\textrm{max} \cdot \delta
,
\end{align*}
where the second to last line follows by the Cauchy-Schwartz inequality.
\end{proof}

Using this, we can prove our main claim of this section.

\begin{lemma}[Deterministic projections]
Let $\vt_1\supr{1}, \dots, \vt_n\supr{1}$ be the result of simultaneously diagonalizing $n $ random projections $T(I,I,\vt_i\supr{1})$ for $i=1,\dots,n$ of tensor $T$, where each $\vt_i\supr{0}$ satisfies $||\vt_i\supr{0} - v_i|| \leq \delta$. For some permutation $\pi$, with probability $1-\delta$, we have
$$ ||\vt_i\supr{1} - v_{\pi(i)}||_2 \leq \frac{\e \cdot C \cdot \kappa}{1 - \sqrt{2} \pi_\textrm{max} \delta} + o(\e). $$
\end{lemma}

\begin{proof}
By the previous lemma, and our assumption on $\e$, we have for all $i, j$,
$$ \vt_i^\top (\pi_i v_i - \pi_j v_j) \geq 1 - \sqrt{2}\cdot\pi_\textrm{max} \cdot \delta. $$

Using our previous bound,
we obtain
\begin{align*}
|| \vt_i - v_i ||_2 
& \leq \e \cdot C \cdot \kappa \cdot \max_{j \neq i} \min_{l=1}^{n} \frac{1}{| \vt_l\supr{0})^\top (\pi_i v_i - \pi_j v_j)|} + o(\e) \\
& \leq \e \cdot C \cdot \kappa \cdot  \max_{j \neq i} \frac{1}{| (\vt_i\supr{0})^\top (\pi_i v_i - \pi_j v_j)|} + o(\e) \\
& \leq \frac{\e \cdot C \cdot \kappa}{1 - \sqrt{2} \pi_\textrm{max} \delta} + o(\e)
.
\end{align*}

\end{proof}

\subsection{Algorithm analysis}

Using the above lemmas, we can easily analyze the performance of our algorithm.

\begin{theorem}
Suppose that $ \e < (\pi_\textrm{min}) / (\pi_\textrm{max} 4\sqrt{2} C \kappa \sqrt{d}). $
At the second step of the algorithm, for some permutation $\pi$, with probability $1-\delta$,
$$ ||\vt_i\supr{1} - v_{\pi(i)}||_2 \leq \frac{\e \cdot C \cdot \kappa}{1/2 - o(\e)} + o(\e). $$
\end{theorem}

\begin{proof}
Follows immediately from applying the above two lemmas.
\end{proof}

To prove a result for eigenvalues, we first need this lemma.

\begin{lemma}[Bauer-Fike]\label{lem:bauer_fike}
Let $M$ be a $d \times d$ matrix. The eigenvalues of a perturbed matrix $M + R$ lie in the union of the disks $\mathcal D_i$ for $1 \leq i \leq d$,w here $\mathcal D_i$ has center $\lambda_i$ and radius at most $||R||_2$.
\end{lemma}

\begin{theorem}
Suppose that $ \e < (\pi_\textrm{min}) / (\pi_\textrm{max} 4\sqrt{2} C \kappa \sqrt{d}). $
At the second step of the algorithm, for some permutation $\pi$, with probability $1-\delta$,
$$ ||\pit_i\supr{1} - \pi_{\pi(i)}||_2 \leq \left( 1 + \frac{ C \cdot \kappa \cdot \pi_i}{1/2 - o(\e)} \right) \e + o(\e). $$
\end{theorem}

\begin{proof}
Recall from the previous theorem that
$$ ||\vt_i\supr{1} - v_{\pi(i)}||_2 \leq \frac{\e \cdot C \cdot \kappa}{1/2 - o(\e)} + o(\e). $$

Recall also that $\pit_i$ is the $i$-th eigenvalue of matrix $M_i\supr{1}$, which is of the form
$$ M_i\supr{1} = \sum_{i=1}^n \pi_i (\vt_i^\top v_i) v_i v_i^\top + R, $$
where $|| R ||_2 < \e$. Therefore $\pit_i = \pi_i (\vt_i^\top v_i)$.

Observe that
\begin{align*}
|| \pi_i - \pi_i \vt_i^\top v_i ||_2
& = || \pi_i - \pi_i (v_i - (v_i - \vt_i))^\top v_i) ||_2 \\
& = || (v_i - \vt_i)^\top v_i \pi_i ||_2 \\
& \leq \frac{\e \cdot C \cdot \kappa \cdot \pi_i}{1/2 - o(\e)} + o(\e)
.
\end{align*}

Let $\lambda_i = \pi_i (\vt_i^\top v_i)$ and let $\pit_i$ be obtained from the eigendecomposition of $M_i\supr{1}$. Combining all of the above, we get that
\begin{align*}
|| \pit_i - \pi_{\pi(i)} ||_2
& \leq || \pit_i - \lambda_i ||_2 + || \lambda_i - \pi _{\pi(i)} ||_2 \\
& \leq \e + \left( \frac{ C \cdot \kappa \cdot \pi_i}{1/2 - o(\e)} \right) \e + o(\e)
,
\end{align*}
where we used the Bauer-Fike lemma to found the first term, and our above analysis to bound the second term.
\end{proof}

\subsection{
